# Supplementary material for: Agent3D-Zero: An Agent for Zero-shot 3D Understanding
Source: arXiv:2403.11835 source file (2024-03-18)
Supplement: Supplementary file 1 [file X-supplement.tex]

\clearpage
\setcounter{page}{1}
% \maketitlesupplementary
\newpage
       % \twocolumn[
       
% \centering{
{\Large{
\centering{
\textbf{Agent3D-Zero:  An Agent for 
   Zero-shot 3D Understanding}\\
\vspace{0.5em}Supplementary Material \\
        \vspace{1.0em}
       % ] %< twocolumn
       }
       }}

\appendix

\setcounter{figure}{0}

\setcounter{table}{0}

This supplementary material is made up of two sections.
% In Section~\ref{sec:additional_visualization}, 
First, we visualize more examples to help intuitively present the question answering (QA) and 3D-assisted dialog results.
Then, we provide the project page including the video that presents our pipeline and demos to further validate the effectiveness of our proposed method. The project page is in the attachment.

% \section{Additional Qualitative Results}
% \label{sec:additional_visualization}
In our main manuscript, we only visualize two tasks on one scene due to the limitation of pages. Here, we add more qualitative examples in Figure~\ref{fig:supplement_example2} to help intuitively present the reasoning results of our method. From the visualized results, it can be seen that our proposed method is able to answer the questions accurately according to the selected images of the specific scene. Meanwhile, the 3D-assisted dialog is presented at the bottom of the figure. These examples vividly demonstrate Agent3D-Zero's adeptness at accurately identifying and describing detailed objects and their relationships within specific 3D environments. Through an intelligent analysis of the scene informed based on the selected images, Agent3D-Zero showcases its remarkable ability to analyze and summarization multiple objects' information and provide precise answers, underscoring its advanced 3D reasoning capabilities.
\begin{figure}[h]
  \centering
  \includegraphics[width=0.8\linewidth]{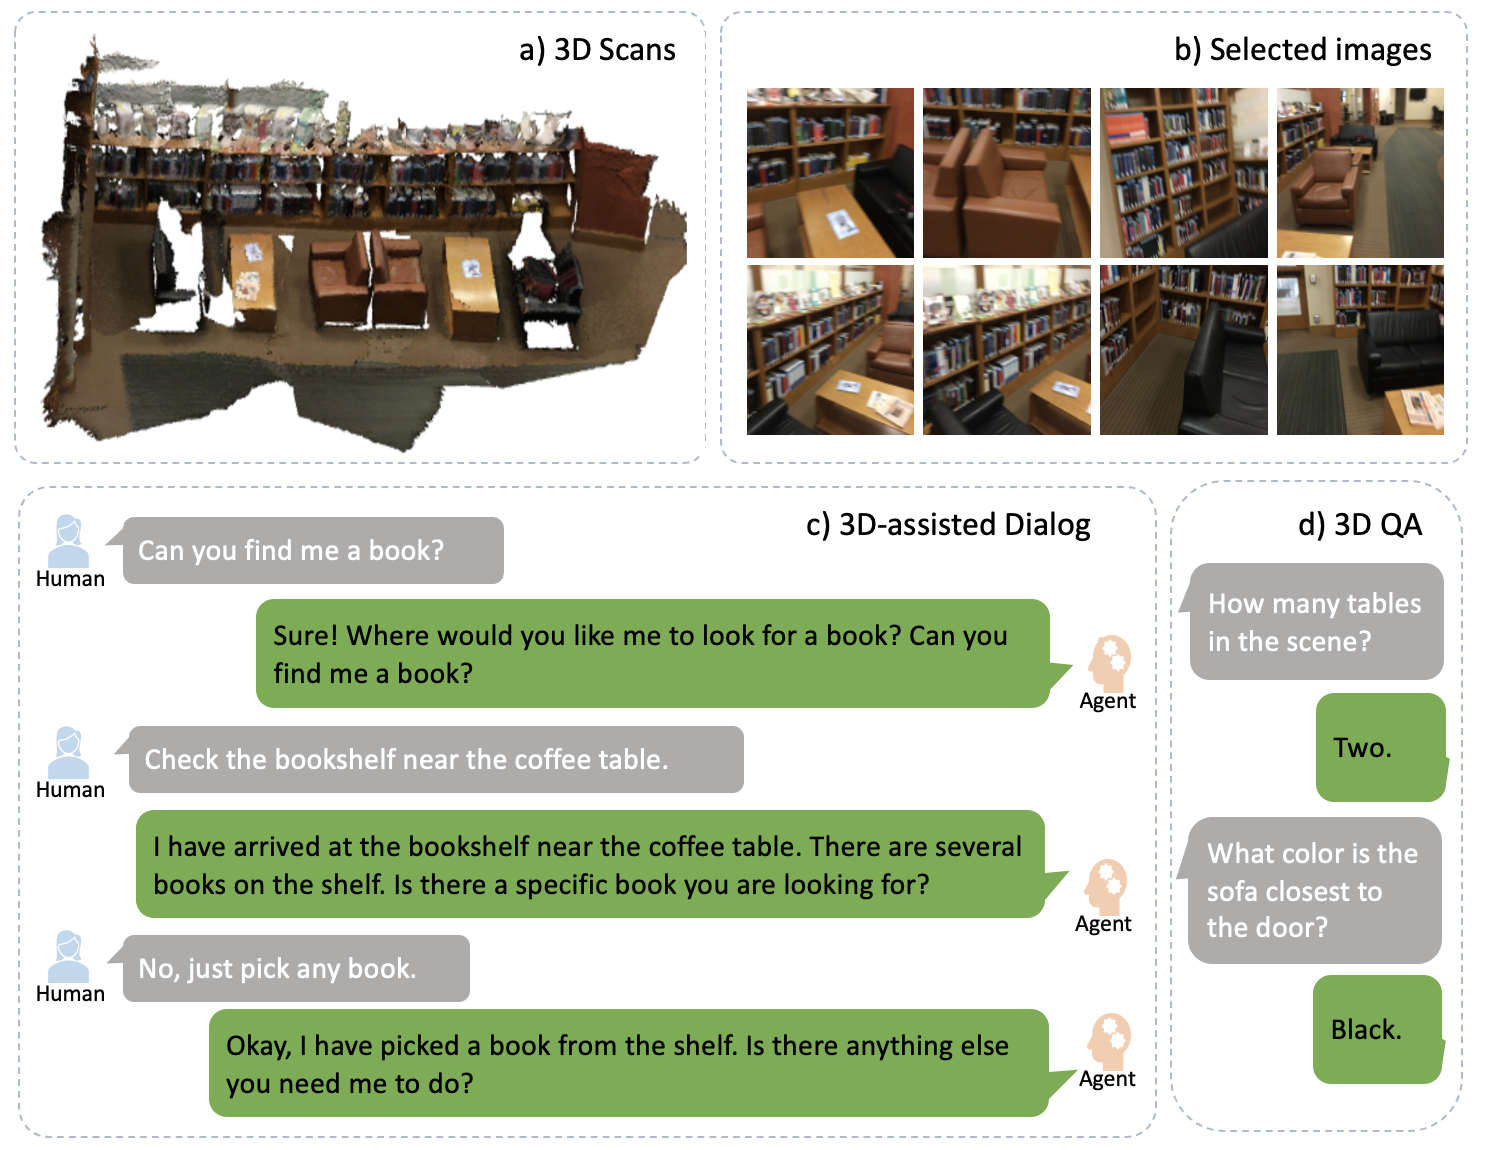}
  \vspace{-0.3cm}
  \caption{
  \textbf{Supplement of Qualitative results on QA and 3D-assisted dialog. } The top presents the 3D scan of a reading room and part of the images selected from different viewpoints. We show examples of 3D-assisted dialog and 3D QA at the bottom.}
  \label{fig:supplement_example2}
  \vspace{-0.3cm}
\end{figure}

% % 
% Having the supplementary compiled together with the main paper means that:
% % 
% \begin{itemize}
% \item The supplementary can back-reference sections of the main paper, for example, we can refer to \cref{sec:intro};
% \item The main paper can forward reference sub-sections within the supplementary explicitly (e.g. referring to a particular experiment); 
% \item When submitted to arXiv, the supplementary will already included at the end of the paper.
% \end{itemize}
% % 
% To split the supplementary pages from the main paper, you can use \href{https://support.apple.com/en-ca/guide/preview/prvw11793/mac#:~:text=Delete%20a%20page%20from%20a,or%20choose%20Edit%20%3E%20Delete).}{Preview (on macOS)}, \href{https://www.adobe.com/acrobat/how-to/delete-pages-from-pdf.html#:~:text=Choose%20%E2%80%9CTools%E2%80%9D%20%3E%20%E2%80%9COrganize,or%20pages%20from%20the%20file.}{Adobe Acrobat} (on all OSs), as well as \href{https://superuser.com/questions/517986/is-it-possible-to-delete-some-pages-of-a-pdf-document}{command line tools}.
